# Supplementary material for: MUTE: Data-Similarity Driven Multi-hot Target Encoding for Neural Network Design
Source: arXiv:1910.07042 source file (2019-10-15)
Supplement: Supplementary file 1 [file appendix.tex]

\subsection{Related Work on Target Encoding}

Target Encoding in the context of Error-Correcting Output Codes (ECOC) has been extensively studied in ~\cite{dietterich1994solving, langford2005sensitive, kuncheva2005using, deng2010applying, rodriguez2018beyond} where such ECOC concept is applied to represent output labels. While  these approaches benefit from the error-correcting capability (as in \prjname ), they are not optimized for a given task or dataset. Unlike \prjname , they do not capture the inherent distributions in the dataset, specifically the relationships between classes, thus not necessarily increasing the predictive power of a neural network model. For example, \cite{yang2015deep} used Hadamard codes to learn deep representations and showed that such presentations are more separable than features learned with 1-of-K encodings, but did neither extract nor utilize the useful information in the dataset.  

Also, there is recent interest in exploring alternatives to one-hot encoding for multi-class classification problems with a focus on improving the performance against adversarial examples. In the multi-way encoding method~\cite{kim2019multiway}, the authors proposed to use datatset-oblivious Random Orthogonal (RO) encodings generated by Gram-Schmidt orthogonalization to reduce the correlation between gradients of the target model and substitute model used by an adversary, and claimed that multi-way encoding trained with mean square error loss and adversarial training increases robustness against adversarial attacks. RO encodings are in real-numbers and have larger encoding dimension than the number of output classes, whereas \prjname  has Hamming codes with the same encoding dimension as the number of output classes. Please note that a larger encoding dimension increases the number of weights that need to be trained.

\subsection{Experimental Results}
Here we tabulate the results obtained in experiments described in Section~\ref{sec:mute_exp}.

\begin{table}[h]
	\centering
	\resizebox{\textwidth}{!}{%
		\begin{tabular}{|c|c|c|c|c|c|c|}
			\hline
			\multirow{2}{*}{\begin{tabular}[c]{@{}c@{}}CNN\\ Arch.\end{tabular}} & \multirow{2}{*}{\begin{tabular}[c]{@{}c@{}}Target \\ Encoding\end{tabular}} & \multicolumn{5}{c|}{Accuracy on Test Datasets}                          \\ \cline{3-7} 
			&                                                                             & Original & Negative & Avg. Blur & Avg. Salt \& Pepper Noise & Avg. FGSM \\ \hline
			\hline
			\multirow{8}{*}{LeNet}                                               & 1-hot                                                                       & \textbf{99.27}    & 24.07    & 98.39     & \textbf{98.81}                     & 98.61     \\ \cline{2-7} 
			& 3-hot                                                                       & 99.09    & 31.29    & 98.30     & 98.62                     & 98.65     \\ \cline{2-7} 
			& 4-hot                                                                       & 99.10    & 25.06    & 98.33     & 98.55                     & 98.79     \\ \cline{2-7} 
			& Weighted 3-hot                                                              & 99.14    & \textbf{44.68}    & 98.46     & 98.63                     & 98.70     \\ \cline{2-7} 
			& Weighted 4-hot                                                              & 99.12    & 43.41    & 98.55     & 98.61                     & 98.67     \\ \cline{2-7} 
			& H-63                                                                        & 99.10    & 29.11    & 98.58     & 98.61                     & \textbf{98.81}     \\ \cline{2-7} 
			& H-127                                                                       & 99.18    & 34.23    & 98.53     & 98.07                     & 98.78     \\ \cline{2-7} 
			& H-255                                                                       & 99.11    & 30.55    & \textbf{98.62}     & 98.59                     & 98.75     \\ \hline
			\hline
			\multirow{8}{*}{ConvNet}                                             & 1-hot                                                                       & 99.10    & 32.20    & 80.37     & 97.49                     & 98.51     \\ \cline{2-7} 
			& 3-hot                                                                       & 98.90    & 42.74    & 97.10     & \textbf{98.63}                     & 98.50     \\ \cline{2-7} 
			& 4-hot                                                                       & 99.01    & 39.58    & 96.68     & 98.17                     & 98.68     \\ \cline{2-7} 
			& Weighted 3-hot                                                              & \textbf{99.14}    & \textbf{50.92}    & 97.09     & 98.38                     & \textbf{98.81}     \\ \cline{2-7} 
			& Weighted 4-hot                                                              & 99.10    & 41.05    & 96.80     & 98.35                     & 98.75     \\ \cline{2-7} 
			& H63                                                                         & 98.88    & 31.08    & 96.71     & 98.34                     & 98.48     \\ \cline{2-7} 
			& H-127                                                                       & 98.92    & 19.98    & 97.13     & 98.07                     & 98.55     \\ \cline{2-7} 
			& H-255                                                                       & 98.89    & 36.50    & \textbf{97.46}     & 98.22                     & 98.50     \\ \hline
		\end{tabular}%
	}
\caption{LeNet and ConvNet architectures with different target encodings were trained on original images in the MNIST training dataset and tested on original and noisy versions of the MNIST test dataset. The proposed multi-bit target encoding method has better average test performance than one-hot encoding or Hadamard encoding (H-63, H-127, and H-255).}
\label{tab:mnist}
\end{table}

\begin{table}[h]
	\centering
	\resizebox{\textwidth}{!}{%
		\begin{tabular}{|c|c|c|c|c|c|}
			\hline
			\multirow{2}{*}{\begin{tabular}[c]{@{}c@{}}CNN\\ Arch.\end{tabular}} & \multirow{2}{*}{\begin{tabular}[c]{@{}c@{}}Target\\ Encoding\end{tabular}} & \multicolumn{4}{c|}{Accuracy on Test Datasets}              \\ \cline{3-6} 
			&                                                                            & Original & Negative & Avg. Blur & Avg. Salt \& Pepper Noise \\ \hline
			\hline
			\multirow{8}{*}{AlexNet}     & 1-hot           & 55.63    & 12.34    & 44.47     & 39.04                     \\ \cline{2-6} 
			& 3-hot                                                                      & 77.25    & 25.88    & 62.31     & 45.95                     \\ \cline{2-6} 
			& 4-hot                                                        & 77.27    & \textbf{29.29}    & 63.09     & 46.05                     \\ \cline{2-6} 
			& Weighted 3-hot                                                             & 76.71    & 26.32    & 62.97     & 47.45                     \\ \cline{2-6} 
			& Weighted 4-hot                                               & 76.76    & 28.87    & 63.26     & \textbf{48.08}                     \\ \cline{2-6} 
			& H-63                                                                       & 78.36    & 24.80    & 63.25     & 47.86                     \\ \cline{2-6} 
			& H-127                                                 & \textbf{78.69}    & 27.32    & \textbf{64.19}     & 47.15                     \\ \cline{2-6} 
			& H-255                                                                      & 78.23    & 23.78    & 59.28     & 43.10                     \\ \hline
			\hline
			\multirow{8}{*}{DenseNet}        & 1-hot                   & \textbf{88.98}    & 46.50    & 52.53     & 34.10                     \\ \cline{2-6} 
			& 3-hot                                                                      & 87.34    & 46.11    & 52.98     & 38.34                     \\ \cline{2-6} 
			& 4-hot                                                                      & 87.44    & 48.85    & 54.33     & 39.19                     \\ \cline{2-6} 
			& Weighted 3-hot                                                             & 86.81    & 49.31    & 55.79     & 39.03                     \\ \cline{2-6} 
			& Weighted 4-hot                              & 86.58    & \textbf{50.43}    & \textbf{57.80}     & \textbf{45.51}         \\ \cline{2-6} 
			& H-63                                                                       & 87.08    & 40.81    & 54.04     & 36.70                     \\ \cline{2-6} 
			& H-127                                                                      & 86.87    & 44.42    & 35.98     & 30.83                     \\ \cline{2-6} 
			& H-255                                                                      & 85.90    & 39.12    & 49.75     & 42.65                     \\ \hline
			\hline
			\multirow{8}{*}{ResNet}      & 1-hot                    & \textbf{83.30}    & 39.55    & 52.21     & 43.96                     \\ \cline{2-6} 
			& 3-hot                                                                      & 80.76    & 38.25    & 52.74     & 46.22                     \\ \cline{2-6} 
			& 4-hot                                                                      & 81.34    & 41.68    & 55.51     & 47.46                     \\ \cline{2-6} 
			& Weighted 3-hot                                                             & 80.91    & 42.18    & 55.99     & 50.22                     \\ \cline{2-6} 
			& Weighted 4-hot                                   & 80.62    & \textbf{44.21}    & \textbf{58.52}     & \textbf{51.27}          \\ \cline{2-6} 
			& H-63                                                                       & 81.48    & 42.31    & 51.47     & 48.98                     \\ \cline{2-6} 
			& H-127                                                                      & 82.11    & 43.27    & 52.30     & 47.66                     \\ \cline{2-6} 
			& H-255                                                                      & 80.70    & 34.92    & 50.42     & 43.13                     \\ \hline
			\hline
			\multirow{8}{*}{ResNeXt}      & 1-hot          & 89.85    & 47.57    & 52.72     & 39.18                     \\ \cline{2-6} 
			& 3-hot                                                       & 89.87    & 49.88    & 51.67     & 34.11                     \\ \cline{2-6} 
			& 4-hot                                                       & 89.61    & 51.27    & 60.35     & 42.31                  \\ \cline{2-6} 
			& Weighted 3-hot                                       & 89.26    & 46.66    & 63.58     & 41.09                     \\ \cline{2-6} 
			& Weighted 4-hot                                       & 89.21    & 47.31    & \textbf{63.88}     & \textbf{42.39}                     \\ \cline{2-6} 
			& H-63                                                       & \textbf{89.89}    & \textbf{52.27}    & 60.12     & 33.63                     \\ \cline{2-6} 
			& H-127                                                      & 89.66    & 44.34    & 46.48     & 40.49                     \\ \cline{2-6} 
			& H-255                                                      & 89.30    & 43.11    & 54.83     & 36.31                     \\ \hline
		\end{tabular}%
	}
\caption{CNN architectures with different target encodings were trained on original images in the CIFAR-10 training dataset and tested on original and noisy versions of the CIFAR-10 test dataset. The proposed multi-bit target encoding method has better average test performance than one-hot encoding or Hadamard encoding (H-63, H-127, and H-255).}
\label{tab:cifar-10}
\end{table}

\begin{table}[h]
	\centering
	\resizebox{\textwidth}{!}{%
		\begin{tabular}{|c|c|c|c|c|c|}
			\hline
			\multirow{2}{*}{\begin{tabular}[c]{@{}c@{}}CNN\\ Arch.\end{tabular}} & \multirow{2}{*}{\begin{tabular}[c]{@{}c@{}}Target\\ Encoding\end{tabular}} & \multicolumn{4}{c|}{Accuracy on Test Datasets}              \\ \cline{3-6} 
			&                                                                            & Original & Negative & Avg. Blur & Avg. Salt \& Pepper Noise \\ \hline
			\hline
			\multirow{5}{*}{AlexNet}                                             & 1-hot                                                                      & 60.04    & 7.09     & 53.43     & 31.22                     \\ \cline{2-6} 
			& 15-hot                                                                     & 83.02    & 10.54    & 78.72     & 40.41                     \\ \cline{2-6} 
			& 20-hot                                                                     & 83.67    & 10.64    & 77.05     & 38.59                     \\ \cline{2-6} 
			& Weighted 15-hot                                                            & \textbf{86.46}    & \textbf{12.49}    & 79.32     & \textbf{45.36}                     \\ \cline{2-6} 
			& Weighted 20-hot                                                            & 86.26    & 12.29    & \textbf{79.95}     & 39.09                     \\ \hline
			\hline
			\multirow{5}{*}{DenseNet}    & 1-hot   & \textbf{95.50}    & 16.38    & \textbf{87.59}     & 22.10                     \\ \cline{2-6} 
			& 15-hot                                                         & 91.96    & \textbf{20.13}    & 79.67     & 28.82                     \\ \cline{2-6} 
			& 20-hot                                                                     & 91.91    & 15.53    & 82.94     & 27.92                     \\ \cline{2-6} 
			& Weighted 15-hot                                                            & 92.31    & 16.08    & 81.00     & 29.47                     \\ \cline{2-6} 
			& Weighted 20-hot                                                            & 91.16    & 19.38    & 82.47     & \textbf{32.24}                     \\ \hline
			\hline
			\multirow{5}{*}{ResNet}            & 1-hot      & \textbf{92.86}    & 13.39    & \textbf{85.02}     & 21.61                     \\ \cline{2-6} 
			& 15-hot                                                                & 89.31    & 19.28    & 82.75     & 26.88                     \\ \cline{2-6} 
			& 20-hot                                                                & 89.71    & 21.33    & 84.17     & 27.63                     \\ \cline{2-6} 
			& Weighted 15-hot                                                & 89.66    & 20.03    & 83.47     & 27.42                     \\ \cline{2-6} 
			& Weighted 20-hot                                                & 89.11    & \textbf{25.32}    & 83.60     & \textbf{31.82}                     \\ \hline
			\hline
			\multirow{5}{*}{ResNeXt}                    & 1-hot            & 95.10    & 13.44    & 88.34     & 25.10                     \\ \cline{2-6} 
			& 15-hot                                                          & \textbf{96.60}    & 19.08    & 88.26     & 33.52                     \\ \cline{2-6} 
			& 20-hot                                                              & 96.35    & 19.08    & \textbf{89.71}    & 34.47                     \\ \cline{2-6} 
			& Weighted 15-hot                                                     & 96.30    & 19.98    & 87.49     & 34.34                     \\ \cline{2-6} 
			& Weighted 20-hot                                       & 96.45    & \textbf{22.48}    & 88.76     & \textbf{37.19}                     \\ \hline
		\end{tabular}%
	}
\caption{CNN architectures with different target encodings were trained on original images in the ICON-50 training dataset and tested on original and noisy versions of the ICON-50 test dataset. The proposed multi-bit target encoding method has better average test performance than one-hot encoding.}
\label{tab:icon50_all}
\end{table}
